# Supplementary material for: Machine Unlearning: A Comprehensive Survey
Source: arXiv:2405.07406 source file (2026-04-20)
Supplement: Supplementary file 1 [file appendix1.tex]

\section{Proof of How Sample Similarity Influences Model Difference and Unlearning Auditing} \label{theorey_analysis_of_similarity}

Here, we provide an example to explain how the similarity of the erased and remaining samples influences the unlearning model difference and unlearning auditing.

Let us consider a linear model with parameters $\theta$ and two input vectors $\texttt{v}_1=[v_{1,1},v_{1,2},v_{1,3}]$ and $\texttt{v}_2=[v_{1,1}+\epsilon_1,v_{1,2}+\epsilon_2,v_{1,3}+\epsilon_3]$. If $\epsilon_i$ (for $i \in [1,2,3]$) represents dissimilar difference (could be noise or other dissimilarities), then $\texttt{v}_2$ can be represented by $\texttt{v}_1$ as $\texttt{v}_2=\texttt{v}_1+\epsilon$. If $\epsilon\simeq0$, then $\texttt{v}_2\simeq\texttt{v}_1$. Assume we have a model $\theta_{\texttt{v}_1}$ trained on $\texttt{v}_1$, and then we train it on $\texttt{v}_2$ and achieve 
\begin{equation}
	\begin{aligned}
		\theta_{[\texttt{v}_1,\texttt{v}_2]} &=\theta_{\texttt{v}_1}+\Delta\theta_{\texttt{v}_1}(\texttt{v}_2) \\ 
		&=\theta_{\texttt{v}_1}+\Delta\theta_{\texttt{v}_1}(\texttt{v}_1+\epsilon) \\
		&=\theta_{\texttt{v}_1}+\Delta\theta_{\texttt{v}_1}(\texttt{v}_1)+\Delta\theta_{\texttt{v}_1}(\epsilon).
	\end{aligned}
\end{equation}
Since the linear model $\theta_{\texttt{v}_1}$ is optimized using $\texttt{v}_1$, the $\Delta \theta_{\texttt{v}_1}(\texttt{v}_1)$ will be minimized at the same time, i.e., $\Delta \theta_{\texttt{v}_1}(\texttt{v}_1) \simeq 0$. Now the $\Delta\theta_{\texttt{v}_1}(\texttt{v}_2) \simeq \Delta \theta_{\texttt{v}_1}(\epsilon)$. If the dissimilarity $\epsilon=0$, then the model difference  $\Delta \theta_{\texttt{v}_1}(\texttt{v}_2) = \theta_{[\texttt{v}_1,\texttt{v}_2]}-\theta_{\texttt{v}_1}$ for unlearning $\texttt{v}_2$ from $\theta_{[\texttt{v}_1,\texttt{v}_2]}$ will be approximate to 0, which is hard for reconstructing unique information of $\texttt{v}_2$. If $\epsilon>0$, then we can reconstruct the unique information of $\texttt{v}_2$ that different from $\texttt{v}_1$ using $\Delta \theta_{\texttt{v}_1}(\epsilon)$.

\section{The Experimental Results of Backdoor Verification Can Only Verify Backdoored Samples} \label{b_v_b}

%\subsection{The experimental results of backdoor verification can only verify backdoored samples} \label{b_v_b}

In \Cref{fig_mnistepochaccdrop}, the backdoor triggers can actually only verify whether the backdoored samples are unlearned as the backdoored samples and unlearned normal samples perform differently during unlearning training process. When the accuracy of backdoor samples drops to 0\%, the model accuracy on model data and test data is still around 80\%.

\begin{figure}
	\centering
	\includegraphics[width=0.87\linewidth]{../../../../PycharmProjects/MUV_by_reconstruction/Experiments/On_MNIST/mnist_epoch_acc_drop}
	%	\vspace{-4mm}
	\caption{Approximate unlearning process on $D_u$ and $D_b$. During unlearning, the backdoor accuracy drops to 0\% at the blue Vertical line. Meanwhile, the model accuracy on normal training data $D_u$ and test data is still around 80\%.%, which shows the different performances of $D_u$ and $D_b$.
	}
	\vspace{-2mm} 
	\label{fig_mnistepochaccdrop}
\end{figure}

\section{Proof of \Cref{first_order}} \label{proof_of_theorem_1}

\iffalse
The changes in the model parameters can be expand using the perturbation theory \cite{avrachenkov2013analytic} as:
\begin{equation} \label{expanding_loss}
	\Delta \theta = \theta^{\epsilon}_{D \backslash D_u} - \theta^* = \mathcal{O}(\epsilon)\theta^{(1)} + \mathcal{O}(\epsilon^2)\theta^{(2)} + \mathcal{O}(\epsilon^3)\theta^{(3)} + \cdot \cdot \cdot,
\end{equation}
where each unlearning sample in $D_u$ is up-weighted by a factor of $\epsilon$.  $\theta^{(1)}$ denotes the first-order (in $\epsilon$) perturbation and $\theta^{(2)}$ is the second-order model perturbation.
\fi

%\subsection{Proof of \Cref{first_order}} 
\begin{proof}
	We provide a derivation of the first-order model difference approximation $\Delta \theta \simeq \frac{1}{n-m} H_{\theta^*}^{-1} \sum_{x_u \in D_u} \nabla L (x_u; \theta^*)$ in \Cref{first_order}. %in the context of loss minimization (M-estimation).
	We define that $\theta^*$ minimizes the empirical risk: 
	\begin{equation}
		R(\theta) \overset{\text{def}}{=} \frac{1}{n} \sum_{x_i \in D} L(x_i;\theta),
	\end{equation}
	where $n$ is the size of the training dataset $D$.
	We assume that $R$ is strictly twice-differentiable and convex in $\theta$, thus, we can positively define 
	\begin{equation}
		H_{\theta^*} \overset{\text{def}}{=} \nabla^2 R(\theta^*) = \frac{1}{n} \sum_{x_i \in D} \nabla^2_{\theta} L(x_i;\theta).
	\end{equation}
	When removing an unlearning dataset $D_u$ with size $m$, $\theta^{\epsilon}_{D \backslash D_u}$ will be the optimal parameter set for the interpolated loss function $\mathcal{L}^{\epsilon}_{D \backslash D_u}(\theta)$, as shown in \Cref{loss_of_unlearning}. Due to the first-order stationary condition, we have
	\begin{equation}\label{nabla_loss_of_unlearning}
		\begin{aligned}
			0 = \nabla \mathcal{L}_{D \backslash D_u}^{\epsilon} (\theta^{\epsilon}_{D \backslash D_u})& =  \nabla \mathcal{L}_{\emptyset}(\theta^{\epsilon}_{D \backslash D_u}) \\
			&+\frac{1}{n} ( - \tilde{\epsilon} \sum_{x \in D \backslash D_u} +\epsilon \sum_{x \in D_u}) \nabla L(x;\theta^{\epsilon}_{D \backslash D_u}).
		\end{aligned}
	\end{equation}
	Let $\theta^{\epsilon}_{D \backslash D_u}$ denote the optimal parameters for $\mathcal{L}^{\epsilon}_{D \backslash D_u}$ minimization, and $\theta^*$ denote the optimal parameters trained on $D$. The changes in the model parameters can be expand using the perturbation theory \cite{avrachenkov2013analytic} as:
	\begin{equation} \label{expanding_loss}
		\Delta \theta = \theta^{\epsilon}_{D \backslash D_u} - \theta^* = \mathcal{O}(\epsilon)\theta^{(1)} + \mathcal{O}(\epsilon^2)\theta^{(2)} + \mathcal{O}(\epsilon^3)\theta^{(3)} + \cdot \cdot \cdot,
	\end{equation}
	where each unlearning sample in $D_u$ is up-weighted by a factor of $\epsilon$.  $\theta^{(1)}$ denotes the first-order (in $\epsilon$) perturbation and $\theta^{(2)}$ is the second-order model perturbation. 
	
	The main idea is to use Taylor series for expanding $\nabla \mathcal{L}_{\emptyset}(\theta^{\epsilon}_{D \backslash D_u})$ around $\theta^*$ base on the perturbation series defined in \Cref{expanding_loss} and compare the terms of the same order in $\epsilon$:
	\begin{equation} \label{expanding_loss_delta}
		\nabla \mathcal{L}_{\emptyset}(\theta^{\epsilon}_{D \backslash D_u}) = \nabla \mathcal{L}_{\emptyset}(\theta^*) + \nabla^2 \mathcal{L}_{\emptyset}(\theta^*)(\theta^{\epsilon}_{D \backslash D_u} - \theta^*) + \cdot \cdot \cdot.
	\end{equation}
	Similarly, we can also expand $\nabla L(x;\theta^{\epsilon}_{D \backslash D_u})$ around $\theta^*$ using Taylor series expansion. To derive $\theta^{(1)}$, we expand \Cref{nabla_loss_of_unlearning} and compare the terms with coefficient $\mathcal{O}(\epsilon)$: 
	\begin{equation}
		\begin{aligned}
			&\epsilon \nabla^2 \mathcal{L}_{\emptyset}(\theta^*) \theta^{(1)} \\
			&=\frac{1}{n} (  \tilde{\epsilon} \sum_{x \in D \backslash D_u} - \epsilon \sum_{x \in D_u})  \nabla L(x;\theta^*) \\
			&= \tilde{\epsilon}  \nabla \mathcal{L}_{\emptyset}(\theta^*)  - \frac{1}{n} (  \tilde{\epsilon}  + \epsilon)  \sum_{x\in D_u} \nabla L(x;\theta^*) \\
			& = -\frac{1}{n} (  \tilde{\epsilon}  + \epsilon  )  \sum_{x\in D_u}  \nabla L(x;\theta^*) \\
			& = -\frac{1}{n-m} \epsilon   \sum_{x\in D_u}  \nabla L(x;\theta^*).
		\end{aligned}
	\end{equation}
	$\theta^{(1)}$ is the first-order approximation of the group influence function. $\epsilon \in [-1,0]$ is used for unlearning.
\end{proof}
%(1 - )L(x;\theta)  (1)L(x;\theta)
