# Supplementary material for: Machine Unlearning: A Comprehensive Survey
Source: arXiv:2405.07406 source file (2026-04-20)
Supplement: Supplementary file 2 [file appendix2.tex]

\section{Discussion about Effectiveness of MUA-MD} \label{discussion_about_effectiveness}
After the server prepares and publishes the pre-trained models, the users will easily achieve their unlearning auditing by using the unlearning model difference and their unlearned samples. The MUA-MD scheme with pre-trained auditing models satisfies the previously defined requirements: the ability to audit data removal and unlearning effectiveness, functionality preservation, and unforgeability. 

% PEDR does not need to add any changes to the ML task model $\theta$; hence, it certainly has the best functionality preservation. Here, we only discuss the ability to verify the unlearning effect and the unforgeability. 

\noindent
\textbf{Ability to Auditing Unlearning.} 
By querying the pre-trained models with the unlearned model difference $\Delta \theta_{x_u}$ for an unlearning requested sample $(x_u,y_u)$, it will return the unlearning execution verifying result and the reconstruction similarity. We set the unlearning data removal result as $\gamma = \mathbb{I}( \text{Verifier}(\theta^*, \theta_u, x_{u})=1)$ and the reconstruction similarity as $\delta = \text{sim}(\hat{x_u}, x_u)$. We call the returned result for the unlearning request $(x_u,y_u)$ as $(\gamma, \delta)$-unlearning auditing, which means $\gamma$ data removal verification and $\delta$ erased data extraction similarity. 

%The PEDR solution certainly has the ability to verify the unlearning effect, as the verification scheme is based on the unlearning model difference, which is the only update for the erased samples on the model. An effective unlearning operation must remove the contribution of the erased samples from the trained mode. The corresponding updated model difference will contain information about the erased samples. The proposed PEDR, based on the reconstruction capability of autoencoders, can utilize the model difference to quantify the unlearned information and provide verification for the unlearning effect.

Based on the observation of the $(\gamma,\delta)$-unlearning auditing for different samples, we have found the similarity between the erased samples and the samples in the remaining dataset influences the unlearning verification significantly. 
Greater similarity leads to a less pronounced unlearning model difference, i.e., a smaller unlearning extent, which diminishes both the unlearning execution inference and unlearning effectiveness reconstruction. By contrast, greater dissimilarity leads to a more pronounced unlearning model difference, ensuring more information about the erased samples to infer and reconstruct, enhancing the auditing effects. This phenomenon is theoretically analyzed in Appendix~\ref{theorey_analysis_of_similarity}, and our experiments confirm the analysis in \Cref{adding_noise}.

\noindent
\textbf{Functionality Preservation.} 
Assume the model with an auditing module $\theta_{\texttt{A}}$, then by the definition, for a classifying ML task, the model $\theta_{\texttt{A}}$ in total will error at most $\epsilon$,
\begin{equation}
	\Pr_{(x,y) \in D} [\theta_{\texttt{A}} \not = y] \leq \epsilon.
\end{equation}
Most existing unlearning auditing methods are based on adding backdoored samples during model training, which easily causes a huge decrease in model utility. However, MUA-MD based on pre-trained models is independent of the original model training period. Therefore, it will not influence the utility of the service model.

%	\forall x \in \mathcal{X}, d(\theta(x), \theta_{\texttt{V}}(x)) \leq \delta.

\noindent
\textbf{Unforgeability.} 
The MUA-MD scheme achieves unforgeability from two key aspects. First, the result with high value $(\gamma, \delta)$-unlearning auditing cannot be forged. Second, the result with minimal value $(\gamma, \delta)$-unlearning auditing correctly answers that similar samples like the erased samples still exist in the remaining dataset.

Firstly, since the Verifier and Reconstructor of MUA-MD are trained and published before receiving unlearning requests, it guarantees the auditing models are trained based on the model point of $\theta^*$ and cannot be changed for later specific unlearning requests. This can be easily checked using timestamping techniques \cite{just1998some,tas2023interchain}. 
If the $(\gamma,\delta)$-unlearning auditing is a high value, it means the later updating unlearning difference contains sufficient information about the erased samples. \textit{Can the server forge a learning update that contains information about the erased data based on the current model point $\theta^*$ to replace the unlearning model difference?} 
The answer is no because the erased data has already undergone minimization through $\theta^*$. Continuing to learn similar samples cannot outcome a pronounced model update for the auditing models of MUA-MD, which is consistent with the analysis in Appendix~\ref{theorey_analysis_of_similarity}. Auditing based on a learning update of the erased samples at the trained model $\theta^*$ will achieve a small value $(\gamma, \delta)$-unlearning auditing result.

Secondly, the MUA-MD auditing models outputting a minimal value $(\gamma, \delta)$-unlearning auditing result means the remaining data contains samples similar to the erased data. This result covers the worst situation, i.e., the server has not conducted unlearning. Therefore, we say the minimal value $(\gamma, \delta)$-unlearning auditing result is valid as it correctly answers that there are still samples similar to erased samples contributing to the model.

Additionally, the MUA-MD solution not only prevents forging attacks \cite{thudi2022necessity} by previously training the auditing models before unlearning requests come but also, to some extent, explains why these attacks can forge an unlearned model. Based on the influence analysis of erased data similarity in Appendix~\ref{theorey_analysis_of_similarity}, if the training dataset contains other similar samples like the erased samples, it would be easy to forge an unlearned model, as many similar samples would provide replaceable contributions to the model. However, if the erased samples are unique and the training data contains no similar samples and features, it would be hard to forge an unlearned model for the erased samples. We believe this finding will benefit the forging attack studies and forging defending studies in machine unlearning.

\section{Impact of ML Task Type} \label{task_impact}

During the training structure of MT-IB in \Cref{fig_choosingmiddlelayer}, the Markov chain of classifying task is established as $i:(X,Y) \to Z \to \hat{Y}$. The Markov chain of autoencoding task is established as $i:(X,Y) \to Z \to \hat{X}$. Due to the Markov chain principle, once information is lost in one layer, it cannot be regained in subsequent layers. This process can be described using mutual information as 
\begin{equation} \label{mutual_Markov}
	\begin{aligned}
		&\textbf{Classifying task:}	&I(X;Y) \geq I(Z;Y) \geq I(\hat{Y},Y) \\
		&\textbf{Autoencoding task:} &I(X;X) \geq I(Z;X) \geq I(\hat{X},X).\\
	\end{aligned}
\end{equation}

Assume we have a task $T$, following the Markov chain in the MT-IB model structure, we have $i:(X,T) \to Z \to \hat{T}$. For an effective IB model for task $T$, it needs to learn a representation $Z$ that maximizes the mutual information $I(Z;T)$. According to the Markov chain and the mutual information relationship in \Cref{mutual_Markov}, we have $I(X;T) \geq I(Z;T) \geq I(\hat{T},T)$. Now, we have the reconstruction upper bound from the mutual information perspective is $I(X;T)$. 

When the task is an autoencoding task, the $T$ is to recover $X$, and the model will learn most information about data $X$, hence, achieving the largest mutual information $I(X;X) = H(X)$. When the task $T$ is not related to the data $X$, and the model will learn nothing about $T$ from $X$, hence, achieving the lowest mutual information $I(X;T)=0$.

\begin{figure}[t]
	\centering
	%\hspace{-3mm}
	%\vspace{-2mm}
	\subfloat{    
		\includegraphics[scale=0.4]{../../../../PycharmProjects/MUV_by_reconstruction/Experiments/On_MNIST/Running_time/mnist_rt_sample_size_bar}
	}
	%	\vspace{-2mm}
	\caption{Running time about different $ESS$.}
	\vspace{-2mm}
	\label{evaluation_of_running_time} 
\end{figure}

\begin{figure*}[t]
	\centering
	\includegraphics[width=0.97\linewidth]{../../../../PycharmProjects/MUV_by_reconstruction/Experiments/On_MNIST/Ablation_exp/ablation_exp}
	\vspace{-2mm}
	\caption{Ablation study about the masking and random division strategies of MUA-MD on MNIST. The legends stand for the entire MUA-MD, MUA-MD without (w/o) the masking strategy, MUA-MD w/o random division strategy, and MUA-MD w/o both strategies}
	\vspace{-2mm}
	\label{fig:ablationexp}
\end{figure*}

\begin{figure*}[t]
	\centering
	\includegraphics[width=0.97\linewidth]{../../../../PycharmProjects/MUV_by_reconstruction/Experiments/On_MNIST/Ablation_exp/second_order_compare}
	\vspace{-2mm}
	\caption{Comparison between the first-order and second-order model differences. The legends stand for the first-order and second-order model difference when the erased data is ``In'' or ``Not In'' the remaining dataset.}
	\vspace{-2mm}
	\label{fig:secondordercompare}
\end{figure*}

\section{Additional Ablation Study Experiments} \label{ad_exp}

\subsection{Impact on Efficiency of ESS } \label{appendix_ess_running_time}
This part is the supplementary results of \Cref{impact_of_ess}, and we keep the same setting as \Cref{impact_of_ess}.

\noindent
\textbf{Impact on Efficiency.} 
The main components of the running time of MUA-MD are the model difference generation and the autoencoder training. The running time of the model difference generation is highly related to $\text{\it ESS}$, and the time of autoencoder training is highly related to the size of the chosen auxiliary dataset for the original training dataset. In our experiments, we randomly select $5\%$ samples on MNIST and CIFAR10 and randomly choose $0.6\%$ samples on CelebA as the auxiliary datasets. This scale of the auxiliary dataset can already guarantee an effective reconstruction and verification performance. 

\Cref{evaluation_of_running_time} shows the training time of MUA-MD and MIB on three datasets. The running time of MUA-MD has a slight decrease as $\text{\it ESS}$ increases. The reason is that when $\text{\it ESS}=1$, MUA-MD needs to generate the model difference for each sample of the auxiliary dataset, which consumes more time than generating one update for multiple samples. For MIB, the running time has no obvious variations when $\text{\it ESS}$ increases. This is because the MIB verification preparation is accompanied by the original model training, which is heavily related to the size of training datasets and epochs. 
MUA-MD has a much more efficient running time compared with MIB, as MUA-MD is independent of the original model training.

\begin{tcolorbox}[colback=white, boxrule=0.3mm]
	\noindent \textbf{Takeaway 6.} 
	MUA-MD achieves a significant efficiency improvement, more than $5\times$ suppedup, because MUA-MD is independent of the original ML service model training.
\end{tcolorbox}

\subsection{Impact of Random Division and Masking}

We now evaluate the impact of our designed two strategies, masking and random division, in improving the auditing effect for multi-sample unlearning scenarios. 
Since these two strategies are conducted after the model difference generation phase, they will not influence the average UE.
Therefore, we focus on the reconstruction similarity, verifiability, and running time.  

\noindent
\textbf{Setup.}
We conduct the experiments on MNIST in four method situations. ``MUA-MD'' means the entire scheme with the two strategies. ``MUA-MD w/o masking'' means we remove the masking strategy of MUA-MD while keeping the random division strategy, and ``MUA-MD w/o division'' means that we remove the random division strategy of MUA-MD while keeping the masking. The ``MUA-MD w/o both'' means we remove both strategies for MUA-MD auditing. The experimental results are presented in \Cref{fig:ablationexp}.

\noindent
\textbf{Reconstruction Similarity to Assess Unlearning Effectiveness.} The first column in \Cref{fig:ablationexp} shows the reconstruction similarity of different methods. All methods achieve a high reconstruction similarity when $\it{ESS} = 1$, which shows the effectiveness of MUA-MD in single-sample unlearning auditing even without the two strategies. However, when the model difference contains information of multiple samples, $\it{ESS} > 1$, if we don't have the random division strategy, the reconstruction similarity drops dramatically, showing as ``MUA-MD w/o division'' and ``MUA-MD w/o both''. The random division plays a vital role in the reconstruction of multiple samples. While the masking strategy does enhance the reconstruction quality, as shown in MUA-MD and ``MUA-MD w/o masking'',  its impact is not as substantial as initially anticipated.

\noindent
\textbf{Verifiability of Data Removal.} Both without masking and without division degrade the verifiability compared with the entire MUA-MD. Moreover, this reduction in verifiability escalates with an increase in $\it{ESS}$.

\noindent
\textbf{Running Time.} Theoretically, removing masking and division will reduce the running time, but these methods achieve similar running times because the main time consumption is the model difference generation and information reconstruction. These strategies are only two small operations in auditing, which will not influence the running time too much.

\subsection{Impact of first-order and second-order model differences}

Usually, the first-order model difference approximation is effective when the size $m$ of $D_u$ is small. However, when computing the group of many erased samples model difference, the second-order coefficient is in the order of $\frac{m^2}{n^2}$, which can be large when the size of $D_u$ is large. In this situation, we need to take both first-order perturbation $\theta^{(1)}$  and second-order perturbation $\theta^{(2)}$ into account. %Below is the corresponding calculation for second order model difference approximation. 
We present the experiments of the first-order and second-order model differences in \Cref{fig:secondordercompare}.
Theoretically, the MUA-MD of the second-order model difference will perform better than the MUA-MD of the first-order model difference because the second-order model difference approximation includes additional second-order information. In \cite{basu2020second}, the authors conducted experiments to remove 50\% samples to demonstrate the improvement of the second-order influence approximation. 
However, since we only unlearn from 1 to 100 samples, the second-order coefficient in this situation is from $\frac{1}{60000^2}$ to $\frac{100^2}{60000^2}$, which is still very small.  Hence, in this scenario, the impact of the second order is minimal, resulting in similar model performances. % when evaluated from the perspectives of Average UE, reconstruction similarity, and verifiability. From the running time perspective, calculating the second-order model difference takes more time than only calculating the first-order model difference, which is apparent when $\it{ESS}=1$.
