# Supplementary material for: Machine Unlearning: A Comprehensive Survey
Source: arXiv:2405.07406 source file (2026-04-20)
Supplement: Supplementary file 8 [file appendix6.tex]

\subsection{Moments of the Minimum of Draws from a Uniform Distribution}
\label{appendix:minimum_draw}

Let $X_1, ..., X_n$ denote the $n$ draws we make from a uniform distribution $U([a,b])$.
We would like to compute the expectation of the minimum of these draws, denoted as $X_{min,n}=\min_{i\in\{1,\dots,n\}}(X_i)$. 

\noindent{\em Proof:} Our proof follows material found online~\cite{math}.
First recall that the cumulative distribution function of any $X_i$ is $F_{X_i} = \frac{x-a}{b-a}\mathbb{1}_{[a,b]} + \mathbb{1}_{[b,+\infty)}$
We then compute the CDF of $X_{min,n}$:
{\small
\begin{equation}
\begin{aligned}
    F_{X_{min,n}}(x) &= \mathbb{P}(X_{min,n} \leq x)\\
    &= 1-\mathbb{P}(X_{min,n} > x)\\
    &= 1 - \mathbb{P}\left(\bigcap_{i=1}^n{(X_i > x)}\right)\\
    &= 1-\prod_{i=1}^n{\mathbb{P}(X_i > x)}\\
    &= \left(1-\prod_{i=1}^n{\left(1 - \frac{x-a}{b-a}\right)}\right)\mathbb{1}_{[a,b]} + \mathbb{1}_{[b,+\infty)}\\
    &= \left(1-\left(\frac{b-x}{b-a}\right)^n\right)\mathbb{1}_{[a,b]} + \mathbb{1}_{[b,+\infty)}\\
\end{aligned}
\end{equation}}
where the antepenultimate line holds because the draws are independent. We now take the derivative and obtain the density function:
{\small\begin{equation}f_{X_{min,n}}(x) = \frac{n}{b-a} \left(\frac{b-x}{b-a}\right)^{n-1}\mathbb{1}_{[a,b]}\end{equation}}

We compute the first moment of $X_{min,n}$ by using an integration by part:
{\small\begin{equation}
    \label{eq:min}
    \mathbb{E}[X_{min,n}] = \int_{-\infty}^{+\infty} xf_{X_{min,n}}(x) \mathrm{d}x = \frac{na + b}{n+1}
\end{equation}}

Similarly, we can compute the second moment by using two integrations by part (or the first moment of $X_{min,n+1}$):
{\small\begin{equation}
\begin{aligned}
    \label{eq:min_square}
    \mathbb{E}[X_{min,n}^2] &= \int_{-\infty}^{+\infty}{x^2f_{X_{min,n}}(x)\mathrm{d}x}\\
    &= a^2 + \frac{2(b-a)}{n+1}\frac{(n+1)a+b}{n+2}
\end{aligned}
\end{equation}}

\subsection{Batched Time Analysis of Slicing}
\label{appendix:time_slicing_batch}

\noindent{\em Proof:} In the batch setting, we retrain all the slices between the slice $\mathfrak{r}_{min}$ having the minimal index that has been hit after $K$ requests and the $R^{th}$ slice. Since the indices $(\mathfrak{r}_i)_{i \in \{1,\dots,K\}} \sim U(\{1,\dots,R\})$ i.i.d. (we assume the requests to be independent), we can use results of previous sections to compute the moments of $\mathfrak{r}_{min}$. The expected cost becomes:
{\small\begin{equation}\begin{aligned}
    \mathbb{E}[C] 
    &= \frac{2e'D}{R(R+1)}\left(\frac{R(R+1)}{2}\right.\\
    &- \left.\frac{1}{2}\left(1 + \frac{2(R-1)}{K+1}\frac{(K+1)+R}{K+2} - \frac{K+R}{K+1}\right)\right)
\end{aligned}\end{equation}}
